# Supplementary material for: Bandit algorithms: Letting go of logarithmic regret for statistical robustness
Source: arXiv:2006.12038 source file (2020-06-22)
Supplement: Supplementary file 1 [file appendix_fixed_horizon_upper_bounds.tex]

\section*{Appendix for Section 4.4 - Fixed-horizon algorithm $\pi_{\textbf{$\mathcal{G}_{MoM}$}}$ for \textbf{$\mathcal{G}$}}

We first prove property 1 of theorem \ref{mom-main-theorem} which is similar to lemma \ref{mom-conc-inequality} with $\delta=\frac{1}{n^2}$.

\subsection*{Proof of Lemma \ref{mom-conc-inequality}}

We first use equation 12 of \citet{bubeck} to establish an inequality with empirical estimator
\begin{align*}
    \mathbb{P}\left( \hat{\mu} - \mu > \eta \right) \leq \frac{3B}{N^{\epsilon}\eta^{1+\epsilon}}\\
    \text{where} \quad \hat{\mu} = \frac{1}{N} \sum_{i=1}^{N} X_i
\end{align*}
%\left( \frac{3u}{\delta n^{\epsilon}} \right)^{\frac{1}{1+\epsilon}}
Using this, if we consider Bernoulli random variable $Y_l = \mathbbm{1}_{\hat{\mu}_l > \mu + \eta}$ for $l=1, 2, \dots, k$, the parameter $p$ satisfies
\begin{align*}
    p \leq \frac{3B}{N^{\epsilon}\eta^{1+\epsilon}}
\end{align*}

Choosing $\eta = (12f(t))^{\frac{1}{1+g(t)}}\left( \frac{1}{N} \right)^{\frac{g(t)}{1+g(t)}}$ and for sufficiently large $t$, when $g(t)<\epsilon$ and $f(t)>B$, we get
\begin{align*}
    p &\leq \frac{3B}{N^{\epsilon}(12f(t))^{\frac{1+\epsilon}{1+g(t)}}(\frac{1}{N})^{\frac{g(t)(1+\epsilon)}{1+g(t)}}}\\
    &= \frac{3B}{(12f(t))^{\frac{1+\epsilon}{1+g(t)}} (N)^{\frac{\epsilon-g(t)}{1+g(t)}}}\\
    &\leq \frac{1}{4}
\end{align*}
\alternate{Choosing $\eta = f(t) \left( \frac{1}{N} \right)^{g(t)}$ where $f:\mathbb{N}\rightarrow \mathbb{R}$ and $g:\mathbb{N}\rightarrow \mathbb{R^{+}}$ be an monotonic increasing and monotonic decreasing function respectively. For sufficiently large $t$, when $g(t)(1+\epsilon)<\epsilon$ and $f(t)^{1+\epsilon}>12B$, we get}
\alternate{\begin{align*}
    p &\leq \frac{3B}{N^{\epsilon}f(t)\left(\frac{1}{N}\right)^{g(t)(1+\epsilon)}}\\
    &\leq \frac{1}{4}
\end{align*}}
Finally, using Hoeffding inequality for binomial random variable,
\begin{align*}
    \mathbb{P}\left( \hat{\mu}_M - \mu > (12f(t))^{\frac{1}{1+g(t)}}\left( \frac{1}{N} \right)^{\frac{g(t)}{1+g(t)}} \right) &= \mathbb{P} \left( \sum_{i=1}^{q} Y_i \geq \frac{q}{2} \right) \leq e^{-2q(\frac{1}{2} -p)^2} \leq e^{\frac{-q}{8}}\\
    &=\delta \qquad \text{since $q = \ceil*{8\log\left(\frac{1}{\delta}\right)}$}
\end{align*}

\alternate{\begin{align*}
    \mathbb{P}\left( \hat{\mu}_M - \mu > f(t) \left( \frac{1}{N} \right)^{g(t)} \right) &= \mathbb{P} \left( \sum_{i=1}^{q} Y_i \geq \frac{q}{2} \right) \leq e^{-2q(\frac{1}{2} -p)^2} \leq e^{\frac{-q}{8}}\\
    &=\delta \qquad \text{since $q = \ceil*{8\log\left(\frac{1}{\delta}\right)}$}
\end{align*}}

\subsection*{Proof of Theorem \ref{mom-main-theorem}}

The following proof is similar to the fixed-horizon proof presented in \citet{lattimore2018bandit}.

We define two events
\begin{align*}
    G_1:& \qquad \mu^* < \min_{t\in [n]} \text{ } \textbf{$\mathcal{U}_{\{i^*, u_{i_{t}^{*}}, n\}}$} \\
    G_2:& \qquad \textbf{$\mathcal{U}_{\{i, u_i, n\}}$} < \mu^* 
\end{align*}
Here, $i^*$ denote the optimal arm and $u_i$ is a constant which will be chosen later. We start with proving the following claim.

\textbf{Claim:} If $G_1$ and $G_2$ is both true, then $T_i(n) \leq u_i$

\textbf{Proof:} Assume $T_i(n) > u_i$. Then $\exists t < n$ for which $T_i(t) = u_i$ and $i^{th}$ arm is chosen at $(t+1)^{th}$ round. Then for such $t$ we have

\begin{align*}
    \textbf{$\mathcal{U}_{\{i, u_i, n\}}$} &= \textbf{$\hat{\mu}_{\{i, u_i, n\}}$} + \textbf{$\mathcal{W}_{\{ u_i, n\}}$}\\
    &< \mu^* \quad &\text{(From $G_2$)}\\
    &< \textbf{$\mathcal{U}_{\{i^*, u_{i_{t}^*}, n\}}$} \quad &\text{(From $G_1$)}
\end{align*}
which is a contradiction since $i^{th}$ arm is chosen at $(t+1)$. 

Now,
\begin{align*}
\mathbb{E}[T_i(n)] &= \mathbb{E}[T_i(n) \mathbbm{1}_{\{G_1 \cap G_2\}}] + \mathbb{E}[T_i(n) \mathbbm{1}_{\{G_{1}^c \cup G_{2}^c\}}]\\
 &\leq u_i + n \mathbb{P}(G_{1}^c \cup G_{2}^c)\\
 &\leq u_i + n\mathbb{P}(G_1^c) + n\mathbb{P}(G_2^c)
\end{align*}

Now, we try to upper bound $\mathbb{P}(G_1^c)$ and $\mathbb{P}(G_1^c)$.

\begin{align*}
    \mathbb{P}(G_1^c) &= \mathbb{P}\left(\bigcup_{t\in[n]} \left\{ \mu^* < \textbf{$\mathcal{U}_{\{i^*, u_{i_{t}^*}, n\}}$} \right\} \right) \\
    &\leq \sum_{t=1}^{n} \mathbb{P} \left( \mu^* < \textbf{$\mathcal{U}_{\{i^*, u_{i_{t}^*}, n\}}$} \right) \\
    &\leq n(n^{-2}) = n^{-1}
\end{align*}
Now, to upper bound $\mathbb{P}(G_2^c)$ we add the following constraint on the choice of $u_i$
\begin{align}
    \Delta_i \geq 2\textbf{$\mathcal{W}_{\{u_i, n\}}$}
\end{align}
Now using this constraint we get,
\begin{align*}
    \mathbb{P}(G_2^c) &= \mathbb{P}\left( \hat{\mu}_{\{i, u_i, n\}} - \mu_i \geq \Delta_i - \textbf{$\mathcal{W}_{\{ u_i, n \}}$} \right)\\
    &\leq \mathbb{P}\left( \hat{\mu}_{\{i, u_i, n\}} - \mu_i \geq \textbf{$\mathcal{W}_{\{ u_i, n \}}$} \right)\\
    &\leq n^{-2}
\end{align*}
Now substituting the upper bound of $\mathbb{P}(G_1^c)$ and $\mathbb{P}(G_1^c)$ we obtain,
\begin{align*}
    \mathbb{E}[T_i(n)] \leq u_i + 1 + \frac{1}{n} \leq u_i + 2
\end{align*}
The tightest bound on $\mathbb{E}[T_i(n)]$ is obtained for the minimum $u_i$ satisfying $\Delta_i \geq 2\textbf{$\mathcal{W}_{\{u_i, n\}}$}$ \QEDclosed
