# Supplementary material for: Bandit algorithms: Letting go of logarithmic regret for statistical robustness
Source: arXiv:2006.12038 source file (2020-06-22)
Supplement: Supplementary file 2 [file neurips_appendix_final_8308.pdf]

## A Appendix for Section 3 - Impossibility of logarithmic regret for statistically robust algorithms

This section is devoted to the proof of Theorem 1. The proof is based on the following characterization of instance-dependent lower bounds from Lattimore and Szepesvári [2018] (see Theorem 16.2):

**Theorem 4.** For any algorithm  $\pi$  that is consistent over  $\mathcal{M}^k$ , and instance  $\nu \in \mathcal{M}^k$ ,

$$\liminf_{n \rightarrow \infty} \frac{R_n(\pi, \nu)}{\log(n)} \geq \sum_{i: \Delta_i > 0} \frac{\Delta_i}{d_i(\nu_i, \mu^*, \mathcal{M})},$$

where  $d_i(\nu_i, \mu^*, \mathcal{M}) := \inf_{\nu'_i \in \mathcal{M}} \{D(\nu_i, \nu'_i) : \mu(\nu'_i) > \mu^*\}$ .

The proof of Theorem 1 therefore follows from the following lemma, which shows that  $d_i(\nu_i, \mu^*, \mathcal{M}) = 0$  for all suboptimal arms of any instance  $\nu$  when  $\mathcal{M}$  is  $\mathcal{B}$ ,  $\mathcal{SG}$ ,  $\mathcal{SE}$ , or  $\mathcal{G}$ .

**Lemma 1.** Fix  $\mathcal{M} \in \{\mathcal{B}, \mathcal{SG}, \mathcal{SE}, \mathcal{G}\}$ . For any distribution  $F \in \mathcal{M}$ , and for any  $a > 0$  and  $b > \mu(F)$ , there exists distribution  $F' \in \mathcal{M}$  such that

$$D(F, F') \leq a \quad \text{and} \quad \mu(F') \geq b.$$

*Proof.* We consider the following two cases.

**Case 1:**  $\mathcal{M} \in \{\mathcal{SG}, \mathcal{SE}, \mathcal{G}\}$

If the distribution  $F$  is unbounded from above (i.e.,  $\bar{F}(y) > 0$  for all  $y \in \mathbb{R}$ ), then the claim follows from Lemma 1 in Agrawal et al. [2020]. The idea there is to construct a new distribution  $F'$  such that for a chosen  $y$ , the CDF on the left side is decreased by a factor of  $e^{-a}$  with respect to  $F$ , and rest of the mass is pushed on the right side of  $y$ . Crucially, under this perturbation,  $F'$  remains in  $\mathcal{M}$ , since on both sides of  $y$  only a constant is being multiplied, thus keeping the functional form of the distribution same. The KL-divergence  $D(F, F')$  is always less than  $a$  independent of the choice of  $y$ . However, the mean of  $F'$  can be made arbitrary large by choosing a suitably large value of  $y$ .

On the other hand, if  $F$  is bounded from above, then the argument below (for the case  $\mathcal{M} = \mathcal{B}$ ) can be applied to construct  $F'$  that is also bounded from above, but satisfies the conditions required. (Specifically, the boundedness of the lower end-point of the support is not required for this argument.)

**Case 2:**  $\mathcal{M} = \mathcal{B}$

We construct a new bounded distribution  $F'$  such that the CDF of  $F'$  is  $e^{-a}$  times the CDF of  $F$  over its support. The rest of the probability mass is uniformly distributed starting from the right end-point of the support to an arbitrary point  $v'$ .

Suppose that the support of  $F$  is contained within  $[u, v]$ . Define the CDF of distribution  $F'$  as follows, for  $\gamma \in (0, 1)$  and  $v' > v$ .

$$\begin{aligned} F'(x) &= (1 - \gamma)F(x) & \forall x \leq v \\ F'(x) &= 1 + \gamma \frac{x - v'}{v' - v} & \forall x \in (v, v'] \end{aligned}$$

Now,

$$D(F, F') = \int_u^v \log \left( \frac{dF(x)}{dF'(x)} \right) dF(x) = -\log(1 - \gamma).$$

Choosing  $\gamma = 1 - e^{-a}$  yields  $D(F, F') = a$ . Turning now to the mean of  $F'$ ,

$$\begin{aligned} \mu(F') &= \int_u^{v'} x dF'(x) = (1 - \gamma)\mu(F) + \int_v^{v'} x \frac{\gamma}{v' - v} dx \\ &= (1 - \gamma)\mu(F) + \frac{\gamma}{2}(v' + v) \end{aligned}$$

Clearly,  $\mu(F')$  can be made arbitrarily large by choosing a suitably large  $v'$ .

□

## 357 B Proof of Theorem 2 - Regret Upper Bound for R-UCB

358 We formally prove theorem 2 in this section. The prove is structurally similar to the bandit regret  
 359 proof presented in Bubeck, Cesa-Bianchi, and Lugosi [2013]. We will show regret bound for the two  
 360 cases  $\nu \in \mathcal{SG}^k$ , and,  $\nu \in \mathcal{SE}^k$ .

361 *Proof.* We first prove for  $\nu \in \mathcal{SE}^k$  and then the other case follows.

362 **Case 1**  $\nu \in \mathcal{SE}^k$

363 We define the following three events for any sub-optimal arm  $i$ .

$$\begin{aligned} E_1 : & \quad \mathcal{U}(i^*, T_{i^*}(t-1), t) \leq \mu^* \\ E_2 : & \quad \hat{\mu}(i, T_i(t-1)) > \mu_i + \mathcal{W}(T_i(t-1), t) \\ E_3 : & \quad \Delta_i < 2\mathcal{W}(T_i(t-1), t) \end{aligned}$$

364 where  $T_i(t)$  denotes the number of times  $i^{th}$  arm is pulled till time instant  $t$ . The three events can  
 365 be interpreted as follows. Event  $E_1$  occurs when the upper confidence bound corresponding to the  
 366 optimal arm is less than its actual mean. Event  $E_2$  corresponds to the case when the mean estimator  
 367 of a sub-optimal arm is much more than its actual mean. As we shall see, both  $E_1$  and  $E_2$  are  
 368 low-probability event and its probability can be upper bounded. Finally, event  $E_3$  corresponds to the  
 369 case when the confidence window of arm  $i$  is large. We now prove that one of these event must be  
 370 true when a sub-optimal arm is chosen at time instant  $t$ . Denote  $I_t$  as the arm chosen at time  $t$ .

371 *Claim* If  $I_t = i$ , then one of  $E_1, E_2$  or  $E_3$  is true.

372 To justify this claim, we assume all the three events to be false and then show a contradiction.

373 We have,

$$\begin{aligned} \mathcal{U}(i^*, T_{i^*}(t-1), t) &> \mu^* \\ &= \mu_{i^*} + \Delta_{i^*} \\ &\geq \mu_{i^*} + 2\mathcal{W}(T_{i^*}(t-1), t) \\ &\geq \hat{\mu}(i^*, T_{i^*}(t-1)) + \mathcal{W}(T_{i^*}(t-1), t) \\ &= \mathcal{U}(i^*, T_{i^*}(t-1), t) \end{aligned}$$

374 which is a contradiction since  $I_t \neq i^*$ .

375 We now show a distribution oblivious concentration inequality for each  $\nu \in \mathcal{SE}^k$ . This inequality  
 376 will be useful in upper bounding probability of events  $E_1$  and  $E_2$ .

377 By our choice of algorithm

$$\hat{\mu}(i, u) = \frac{1}{u} \sum_{j=1}^u X_j ; \quad \mathcal{W}(u, t) = \sqrt{\frac{f(t) \log(t)}{u}}$$

378 We assume the underlying distribution to be  $\nu \in \mathcal{SE}(v, \alpha)^k$ . For any confidence width  $\mathcal{W}$ , we have  
 379 the following concentration inequality (see equation 2.18 in Wainwright [2019])

$$\mathbb{P} \left( \frac{1}{u} \sum_{j=1}^u X_j - \mu \geq \mathcal{W} \right) \leq \exp \left( - \min \left\{ \frac{u\mathcal{W}^2}{2v^2}, \frac{u\mathcal{W}}{2\alpha} \right\} \right)$$

We are interested only in small values of the confidence window  $\mathcal{W}$ , and hence the first term in the  
 minimum expression is of interest to us. For the first term to be less than the second term, we have  
 the following inequality

$$\mathcal{W} \leq \frac{v^2}{\alpha}$$

Putting the value of confidence window  $\mathcal{W}(u, t)$  in this inequality, we get,

$$u \geq f(t) \log(t) \left( \frac{\alpha}{v^2} \right)^2$$

380 Denote the minimum  $u$  satisfying this inequality as  $u_0$ . Hence for all  $u > u_0$  we have,

$$\mathbb{P}(\hat{\mu}(i^*, u) + \mathcal{W}(u, t) > \mu^*) \leq \exp\left(\frac{-f(t) \log(t)}{2v^2}\right)$$

381 Since  $f(t)$  is a sub-linearly growing function, for all time  $t > t_0$ , we are guaranteed to have  
 382  $f(t) > 8v^2$ , where  $t_0 = f^{-1}(8v^2)$ . Substituting this inequality in the above expression yields,

$$\mathbb{P}(\hat{\mu}(i^*, u) + \mathcal{W}(u, t) > \mu^*) \leq \exp(-4 \log(t)) = t^{-4}$$

383 This expression establishes a distribution oblivious inequality for subexponential random variables.  
 384 This inequality is valid for all time instances  $t > t_0$  and  $u > u_0$ , where  $t_0$  is a distribution dependent  
 385 constant parameter while  $u_0$  depends on the distribution as well as the choice of  $f$ . In addition,  $u_0$  is  
 386 an increasing function with number of rounds  $t$ .

387 This inequality is useful in establishing an upper bound on the probability of events  $E_1$  and  $E_2$ . We  
 388 have,

$$\mathbb{P}(E_1) \leq \mathbb{P}(\exists u \in [t] : \mathcal{U}(i^*, u, t) \leq \mu^*) \leq t \cdot t^{-4} = t^{-3} \text{ by union bound over } u$$

389 Similarly,  $\mathbb{P}(E_2) \leq t^{-3}$ .

390 Let  $u'_i$  denote the maximum value of  $T_i(t-1)$  for which event  $E_3$  is true. Consequently, for all  
 391  $t > u'_i$  and  $u > u_0$ , if  $I_t = i$ , then at least one of the event  $E_1, E_2$  is true. Finally, we choose  
 392  $u_i = \max(u'_i, u_0, t_0)$  since we wish to apply the above concentration inequality for all time instances  
 393  $t > u_i$ .

394 Now, for any sub-optimal arm  $i$ ,

$$\begin{aligned} \mathbb{E}[T_i(t)] &= \mathbb{E}\left[\sum_{s=1}^t \mathbb{1}\{I_s = i\}\right] \\ &\leq u_i + \mathbb{E}\left[\sum_{s=u_i+1}^t \mathbb{1}\{I_s = i\}\right] \\ &= u_i + \mathbb{E}\left[\sum_{s=u_i+1}^t \mathbb{1}\{I_s = i, E_1 \text{ true or } E_2 \text{ true}\}\right] \\ &\leq u_i + \sum_{s=u_i+1}^t \mathbb{P}(E_1 \cup E_2) \\ &\leq u_i + \sum_{s=u_i+1}^t \frac{2}{s^3} \leq u_i + 4 \end{aligned}$$

395 Evaluating the value of  $u_i$ , we get

$$u_i = \max\left\{\frac{4f(t) \log(t)}{\Delta_i^2}, f(t) \log(t) \left(\frac{\alpha}{v^2}\right)^2, t_0\right\}$$

However, we observe that  $t_0$  is a constant and thus the first two terms ( $u'_i, u_0$ ) will be more than  $t_0$  after a time instance, say  $t_1$ . Hence,

$$\mathbb{E}[T_i(t)] \leq \max\left\{\frac{4f(t) \log(t)}{\Delta_i^2}, f(t) \log(t) \left(\frac{\alpha}{v^2}\right)^2\right\} + 4 \quad \forall t > t_{\min}^{\mathcal{SE}}(\nu)$$

where the instance dependent threshold  $t_{min}^{\mathcal{SE}}(\nu) = \max(t_0, t_1)$ .

Thus, we get the regret upper bound as

$$R_t(\nu) \leq \sum_{i: \Delta_i > 0} \left( f(t) \log(t) \max \left\{ \frac{4}{\Delta_i}, \Delta_i \left( \frac{\alpha}{v^2} \right)^2 \right\} + 4\Delta_i \right) \quad \forall t > t_{min}^{\mathcal{SE}}(\nu)$$

**Case 2**  $\nu \in \mathcal{SG}^k$

We observe that,  $\mathcal{SG}$  is a special case of  $\mathcal{SE}$  with  $\alpha \rightarrow 0$ . And hence, the regret expression can be obtained as

$$R_t(\nu) \leq \sum_{i: \Delta_i > 0} \left( \frac{4f(t) \log(t)}{\Delta_i} + 4\Delta_i \right) \quad \forall t > t_{min}^{\mathcal{SG}}(\nu)$$

where the instance dependent threshold  $t_{min}^{\mathcal{SG}} = \max(t_0, t_1)$  with  $t_0$  and  $t_1$  same as the previous case.

□

### B.1 Regret bounds when $t < t_{min}$

We discuss a weaker regret bound for time instances less than the threshold time  $t_{min}$ . In the proof of theorem 2 above, we use a slow increasing scaling function to make the inequality oblivious to its parameters. However, we are also interested in obtaining a regret bound for  $t < t_{min}$ . We have,

$$\mathbb{P}(\hat{\mu}(i^*, u) + \mathcal{W}(u, t) > \mu^*) \leq \exp(-\hat{c}f(t) \log(t))$$

where

$$\hat{c} = \begin{cases} \frac{2}{(b-a)^2}, & \text{if } \nu \in \mathcal{B}^k \\ \frac{1}{2\sigma^2}, & \text{if } \nu \in \mathcal{SG}^k \\ \frac{1}{2v^2}, & \text{if } \nu \in \mathcal{SE}^k \end{cases}$$

Substituting this weaker concentration bound in the above proof of regret bound we get,

$$\mathbb{E}[T_i(t)] \leq u_i + \sum_{s=u_i+1}^t t^{1-\hat{c}f(t) \log(t)}$$

as the expected number of times a sub-optimal arm is pulled. The above expression for  $\mathbb{E}[T_i(t)]$  still yields a *sub-linear* upper bound, though weaker than before.

## C Proof of Theorem 3 - Regret Upper Bound for R-UCB-G

We prove theorem 3 in this section. This proof is similar to proof of theorem 2 given in appendix B.

*Proof.* We define the following three events for any sub-optimal arm  $i$ .

$$\begin{aligned} E_1 : & \quad \mathcal{U}(i^*, T_{i^*}(t-1), t) \leq \mu^* \\ E_2 : & \quad \hat{\mu}(i, T_i(t-1), t) > \mu_i + \mathcal{W}(T_i(t-1), t) \\ E_3 : & \quad \Delta_i < 2\mathcal{W}(T_i(t-1), t) \end{aligned}$$

where  $T_i(t)$  denotes the number of times  $i^{th}$  arm is pulled till time instant  $t$ . The three events can be interpreted as follows. Event  $E_1$  occurs when the upper confidence bound corresponding to the optimal arm is less than its actual mean. Event  $E_2$  corresponds to the case when the mean estimator of a sub-optimal arm is much more than its actual mean. As we shall see, both  $E_1$  and  $E_2$  are low-probability event and its probability can be upper bounded. Finally, event  $E_3$  corresponds to the

case when the confidence window of arm  $i$  is large. We now prove that one of these event must be true when a sub-optimal arm is chosen at time instant  $t$ . Denote  $I_t$  as the arm chosen at time  $t$ .

*Claim* If  $I_t = i$ , then one of  $E_1, E_2$  or  $E_3$  is true.

To justify this claim, we assume all the three events to be false and then show a contradiction.

We have,

$$\begin{aligned}\mathcal{U}(i^*, T_{i^*}(t-1), t) &> \mu^* \\ &= \mu_i + \Delta_i \\ &\geq \mu_i + 2\mathcal{W}(T_i(t-1), t) \\ &\geq \hat{\mu}(i, T_i(t-1), t) + \mathcal{W}(T_i(t-1), t) \\ &= \mathcal{U}(i, T_i(t-1), t)\end{aligned}$$

which is a contradiction since  $I_t \neq i^*$ .

Now, by our choice of algorithm

$$\hat{\mu}(i, u, t) = \frac{1}{u} \sum_{j=1}^u X_j \mathbb{1}_{\{|X_j| \leq f(t)\}}$$

We attempt to establish a distribution oblivious concentration inequality with mean estimator chosen as  $\hat{\mu}(i, u, t)$ . We draw inspiration from already established non-oblivious concentration inequality based on this mean estimator (see Lemma 1 in Bubeck, Cesa-Bianchi, and Lugosi [2013], Lemma 1 in Yu, Shao, Lyu, and King [2018] which uses results from Seldin, Laviolette, Cesa-Bianchi, Shawe-Taylor, and Auer [2012]).

We assume the underlying instance to be in  $G(\epsilon, B)^k$ . For a truncation parameter  $f(t)$ , we have, with a probability at least  $1 - t^{-4}$

$$\begin{aligned}\mu - \hat{\mu}(i, u, t) &\leq \frac{B}{f(t)^\epsilon} + \frac{1}{u} \left( 2f(t) \log(2t^4) + u \frac{B}{2f(t)^\epsilon} \right) \\ &\leq \frac{3B}{2f(t)^\epsilon} + \frac{16f(t) \log(t)}{u}\end{aligned}$$

Now, the only non-obliviousness is due to the first term. We observe that, for all  $t > t_0$ ,  $3B \log(f(t)) < 2f(t)^\epsilon$ . There always exists  $t_0$  such that this is true, since, left hand side is a sub-linear term, while right hand side is not.

For all  $t > t_0$ , with a probability at least  $1 - t^{-4}$

$$\begin{aligned}\mu - \hat{\mu}(i, u, t) &\leq \frac{1}{\log(f(t))} + \frac{16f(t) \log(t)}{u} \\ \Rightarrow \mathbb{P}(\mu - \hat{\mu}(i, u, t) \geq \mathcal{W}(u, t)) &\leq t^{-4}\end{aligned}$$

This expression establishes a distribution oblivious inequality for a general (even heavy-tailed) random variables. This inequality is valid for all time instances  $t > t_0$ , where  $t_0$  is a distribution dependent constant parameter.

This inequality is useful in establishing an upper bound on the probability of events  $E_1$  and  $E_2$ , similar to case 1 in the proof given in Appendix B. We have,

$$\mathbb{P}(E_1) \leq \mathbb{P}(\exists u \in [t] : \mathcal{U}(i^*, u, t) \leq \mu^*) \leq t \cdot t^{-4} = t^{-3} \text{ by union bound over } u$$

Similarly,  $\mathbb{P}(E_2) < t^{-3}$ .

438 Now, we proceed to obtain regret upper bound similar to case 1 in the proof given in Appendix B.  
 439 We define  $u'_i$  as the maximum value of  $T_i(t-1)$  for which event  $E_3$  is true. Also, we wish to apply  
 440 concentration bound for all time instants  $t > u_i$ . Consequently, we choose  $u_i = \max(u'_i, t_0)$ .  
 441 Similar to the previous case, we get,

$$\mathbb{E}[T_i(t)] \leq u_i + 4$$

442 The value of  $u_i$  can be evaluated from the inequality given in event  $E_3$  and the choice of  $\mathcal{W}(u, t)$ .  
 443 We get,

$$u_i = \max \left\{ \frac{32f(t) \log(t)}{\Delta_i - \frac{2}{\log(f(t))}}, t_0 \right\}$$

444 .

445 However, the above calculated value of  $u'_i$  is valid only when

$$\Delta_i - \frac{2}{\log(f(t))} > 0$$

446 Let  $t_1$  denote the minimum value of  $t$  satisfying the equation above. Moreover, we observe that  $t_0$  is  
 447 a constant and thus the first term in the expression of  $u_i$  will be more than  $t_0$  after a time instance,  
 448 say  $t_2$ . Hence,

$$\mathbb{E}[T_i(t)] \leq \frac{32f(t) \log(t)}{\Delta_i - \frac{2}{\log(f(t))}} \quad \forall t > t_{\min}(\nu)$$

449 where the instance dependent threshold  $t_{\min} = \max(t_0, t_1, t_2)$ .

450 Thus, we get the regret upper bound as

$$R_t(\nu) \leq \sum_{i: \Delta_i > 0} \left( \frac{32f(t) \log(t)}{1 - \frac{2}{\Delta_i \log(f(t))}} + 4\Delta_i \right) \quad \forall t > t_{\min}(\nu)$$

451

□

## 452 **D Robust Upper Confidence Bound algorithm for arbitrary instances using** 453 **Median of Means (MoM) estimator**

454 Similar to R-UCB-G algorithm, we present yet another statistically robust algorithm over  $\mathcal{G}^k$ . Instead  
 455 of truncation-based estimator, we use median of means estimator (see Bubeck et al. [2013]). This  
 456 estimator works well under excessive variability in the sample values. The mean estimator in  
 457 MoM works as follows. The samples are first divided into  $q$  bins each having equal number of  
 458 samples. Empirical mean is calculated for each of the bins and the median of  $q$  mean values is the  
 459 mean estimator of the samples. In truncation-based estimator, high sample values will require high  
 460 truncation value in order to contribute to the mean estimator. For such excessive variable samples,  
 461 the proposed algorithm, R-UCB-G-MoM will have slightly better finite horizon performance.

462 In addition to scaling function  $f$  put down in Definition 1, we need another class of functions in this  
 463 algorithm, which is stated as follows.

**Definition 2.** A function  $g : \mathbb{N} \rightarrow (0, \infty)$  is said to be slow decaying if

$$g(t+1) \leq g(t) \quad \forall t \in \mathbb{N}, \quad \lim_{t \rightarrow \infty} g(t) = 0, \quad \lim_{t \rightarrow \infty} \frac{g(t)}{t^a} = 0 \quad \forall a > 0.$$

464 R-UCB-G-MoM provides the following regret guarantee over instances in  $\mathcal{G}^k$ .

---

**Algorithm 3** R-UCB-G-MoM

---

**Input**  $k$  arms, slow growing scaling function  $f$ , slowly decaying function  $g$

**Initialize**  $\mathcal{R}_i = \{ \}$ ,  $u_i = 0$  for all arm  $i$

**for**  $t = 1$  to  $k$  **do**

pull arm with index  $i = t - 1$  and observe reward  $R_t$

Append  $R_t$  to  $\mathcal{R}_i$  and update  $u_i \leftarrow u_i + 1$

**end for**

**for**  $t = k + 1, k + 2, \dots$  **do**

Calculate mean estimator  $\hat{\mu}(i, u, t)$  using algorithm 4 with input  $\mathcal{R}_i, u_i$  and  $t$

Calculate the upper confidence bound as

$$\mathcal{U}(i, u_i, t) = \hat{\mu}(i, u, t) + \underbrace{f(t) \left( \frac{32 \log(t)}{u} \right)^{g(t)}}_{\mathcal{W}(u_i, t)}$$

Pull arm  $i$  maximizing  $\mathcal{U}(i, u_i, t)$  and observe reward  $R_t$

Append  $R_t$  to  $\mathcal{R}_i$  and update  $u_i \leftarrow u_i + 1$

**end for**

---

---

**Algorithm 4** Function to Calculate Median of Means (MoM)

---

**Input**  $\mathcal{R}, u, t$ .

**if**  $u > 32 \log(t)$  **then:**

Take  $q = \lceil 32 \log(t) \rceil$  and  $N = \lceil \frac{u}{q} \rceil$

Compute  $\hat{\mu}_l = \frac{1}{N} \sum_{m=1}^N R_{\{(l-1)N+m\}}$  for  $l = 1, 2, \dots, q$

**return** median( $\hat{\mu}_1, \hat{\mu}_2, \dots, \hat{\mu}_q$ )

**else:**

**return** median( $\mathcal{R}$ )

**end if**

---

**Theorem 5.** Consider the algorithm R-UCB-G-MoM with a specified slow growing scaling function  $f$  and slow decaying function  $g$ . For an instance  $\nu \in \mathcal{G}(\epsilon, B)^k$ , there exists a threshold  $t_{\min}(\epsilon, B)$  such that for  $t > t_{\min}(\epsilon, B)$ , the regret under R-UCB-G-MoM satisfies

$$R_t(\nu) \leq \sum_{i: \Delta_i > 0} \left( \Delta_i \left( \frac{2f(t)}{\Delta_i} \right)^{\frac{1}{g(t)}} 32 \log(t) + 4\Delta_i \right).$$

465 The proof is similar to proof of theorem 2 presented in appendix B.

466 *Proof.* We define the following three events for any sub-optimal arm  $i$ .

$$\begin{aligned} E_1 : & \quad \mathcal{U}(i^*, T_{i^*}(t-1), t) \leq \mu^* \\ E_2 : & \quad \hat{\mu}(i, T_i(t-1), t) > \mu_i + \mathcal{W}(T_i(t-1), t) \\ E_3 : & \quad \Delta_i < 2\mathcal{W}(T_i(t-1), t) \end{aligned}$$

467 where  $T_i(t)$  denotes the number of times  $i^{th}$  arm is pulled till time instant  $t$ . The three events can  
468 be interpreted as follows. Event  $E_1$  occurs when the upper confidence bound corresponding to the  
469 optimal arm is less than its actual mean. Event  $E_2$  corresponds to the case when the mean estimator  
470 of a sub-optimal arm is much more than its actual mean. As we shall see, both  $E_1$  and  $E_2$  are  
471 low-probability event and its probability can be upper bounded. Finally, event  $E_3$  corresponds to the  
472 case when the confidence window of arm  $i$  is large. We now prove that one of these event must be  
473 true when a sub-optimal arm is chosen at time instant  $t$ . Denote  $I_t$  as the arm chosen at time  $t$ .

474 *Claim* If  $I_t = i$ , then one of  $E_1, E_2$  or  $E_3$  is true.

475 To justify this claim, we assume all the three events to be false and then show a contradiction.

476 We have,

$$\begin{aligned}
\mathcal{U}(i^*, T_{i^*}(t-1), t) &> \mu^* \\
&= \mu_i + \Delta_i \\
&\geq \mu_i + 2\mathcal{W}(T_i(t-1), t) \\
&\geq \hat{\mu}(i, T_i(t-1), t) + \mathcal{W}(T_i(t-1), t) \\
&= \mathcal{U}(i, T_i(t-1), t)
\end{aligned}$$

477 which is a contradiction since  $I_t \neq i^*$ .

Now, by our choice of algorithm  $\hat{\mu}(i, u, t)$  is the *median of means* estimator. In this mean estimator, we first divide the samples into  $q$  bins, and compute the average of all the bins. Each bin will have  $N = \lceil \frac{u}{q} \rceil$  samples. We return the median of these  $q$  bins as the mean estimator. We attempt to establish a distribution oblivious concentration inequality for this mean estimator. Formally, this estimator is defined as

$$\hat{\mu}(i, u, t) = \text{median}(\hat{\mu}_1, \hat{\mu}_2, \dots, \hat{\mu}_q) \quad \text{where } q = \lceil 32 \log(t) \rceil \quad \text{and} \quad \hat{\mu}_l = \frac{1}{N} \sum_{m=1}^N X_{\{(l-1)N+m\}}$$

478 The choice of  $q = \lceil 32 \log(t) \rceil$  is useful in establishing the required concentration inequality. This  
479 requirement comes from the fact that we need at least  $N = 1$  samples per bin. Further, we assume that  
480 for all arms,  $u > 32 \log(t)$ . Hence, the inequality that we now propose is valid only for  $u > 32 \log(t)$ .

We define a bernoulli random variable  $Y_l = \mathbb{1}\{\hat{\mu}_l > \mu + \mathcal{W}\}$ . According to equation 12 in Bubeck, Cesa-Bianchi, and Lugosi [2013],  $Y_l$  has the parameter

$$p \leq \frac{3B}{N^\epsilon \mathcal{W}^{1+\epsilon}}$$

481 Choosing  $\mathcal{W}(u, t) = f(t) \left(\frac{1}{N}\right)^{g(t)}$ , where  $f(t)$  is a slow growing function, and  $g(t)$  is a slow  
482 decaying function, yields,

$$p \leq \frac{3B}{N^\epsilon f(t)^{1+\epsilon} \left(\frac{1}{N}\right)^{g(t)(1+\epsilon)}}$$

483 Since  $f(t)$  is slow growing and  $g(t)$  is slow decaying, we are guaranteed to have a  $t_0$  such that, for  
484 all  $t > t_0$ , we have  $g(t) < \frac{\epsilon}{1+\epsilon}$  and  $f(t)^{1+\epsilon} > 12B$ . For such  $t > t_0$ , we get,

$$p \leq \left(\frac{1}{4}\right) \left(\frac{3B}{12f(t)^{1+\epsilon}}\right) \left(\frac{1}{N^{\epsilon - g(t)(1+\epsilon)}}\right) \leq \frac{1}{4}$$

485 Finally, using Hoeffding inequality for binomial random variable,

$$\begin{aligned}
\mathbb{P}(\hat{\mu}(i, u, t) - \mu > \mathcal{W}(u, t)) &= \mathbb{P}\left(\sum_{j=1}^q X_j\right) \leq \exp\left(-2q\left(\frac{1}{2} - p\right)^2\right) \\
&\leq \exp\left(\frac{-q}{8}\right) = \exp\left(\frac{-32 \log(t)}{8}\right) = t^{-4}
\end{aligned}$$

486 Note that this inequality is valid for all time instances  $t > t_0$  and  $u > u_0$  where  $t_0$  is a distribution  
487 dependent constant parameter and  $u_0 = \lceil 32 \log(t) \rceil$ , an increasing function.

488 This inequality is useful in establishing an upper bound on the probability of events  $E_1$  and  $E_2$ ,  
489 similar to case 1. We have,

$$\mathbb{P}(E_1) \leq \mathbb{P}(\exists u \in [t] : \mathcal{U}(i^*, u, t) \leq \mu^*) \leq t \cdot t^{-4} = t^{-3} \quad \text{by union bound over } u$$



490 Similarly,  $\mathbb{P}(E_2) \leq t^{-3}$ .

491 We define  $u'_i$  as done in the the proof of theorem 2. However, for the above distribution oblivious  
 492 concentration inequality to hold, we have an additional constraint of  $u > u_0$ . Hence, in this case we  
 493 choose  $u_i = \max(u'_i, u_0, t_0)$ .

494 Similar to the previous two cases, we get,

$$\mathbb{E}[T_i(t)] \leq u_i + 4 \quad \text{but here} \quad u_i = \max \left\{ \left( \frac{2f(t)}{\Delta_i} \right)^{\frac{1}{g(t)}} 32 \log(t), 32 \log(t), t_0 \right\}$$

However, we observe that  $t_0$  is a constant and thus the first two terms  $(u'_i, u_0)$  will be more than  $t_0$  after a time instance, say  $t'_1$ . Moreover, the first function is faster growing than the second function, since  $\left( \frac{2f(t)}{\Delta_i} \right)^{\frac{1}{g(t)}}$  is increasing with time instance  $t$ . Denote  $t''_1$  as the threshold time. Define  $t_1 = \max(t'_1, t''_1)$ . Hence,

$$\mathbb{E}[T_i(t)] \leq \left( \frac{2f(t)}{\Delta_i} \right)^{\frac{1}{g(t)}} 32 \log(t) + 4 \quad \forall t > t_{\min}(\nu)$$

495 where the instance dependent threshold  $t_{\min}(\nu) = \max(t_0, t_1)$ .

Thus, we get the regret upper bound as

$$R_t(\nu) \leq \sum_{i: \Delta_i > 0} \left( \Delta_i \left( \frac{2f(t)}{\Delta_i} \right)^{\frac{1}{g(t)}} 32 \log(t) + 4\Delta_i \right) \quad \forall t > t_{\min}(\nu)$$

496 It is left to show that the above regret bound is indeed *consistent*. We show that there exists appropriate  
 497 choices of  $f(t)$  and  $g(t)$  so that the overall regret expression can be made as close to logarithmic as  
 498 we want.  $\square$

499 **Corollary 1.** *For every slow increasing function  $\Phi(t)$ , there exists slow increasing function  $f(t)$ ,  
 500 slow decreasing decreasing  $g(t)$  and  $t_{\min}$  such that  $\forall \Delta_i, t > t_{\min}$*

$$\left( \frac{2f(t)}{\Delta_i} \right)^{\frac{1}{g(t)}} \leq \Phi(t)$$

501 *Proof.* We see that  $e^{0.5(\log \Phi(t))^{1-c}}$  is an increasing function for  $c \in (0, 1)$ . Hence, we choose  
 502  $f(t) = 0.5e^{0.5(\log \Phi(t))^{1-c}}$  and  $g(t) = \frac{1}{\log^c(\Phi(t))}$ . Also there exists  $t_0$  such that for all  $t > t_0$ ,  
 503  $\frac{1}{\Delta_i} \leq e^{0.5(\log \Phi(t))^{1-c}}$  since LHS is a constant while RHS is an increasing function of  $t$ . Thus, we  
 504 have,

$$\frac{f(t)}{\Delta_i} \leq e^{(\log \Phi(t))^{1-c}} \quad \forall t > t_0$$

505 Again, there exists  $t_1$  such that LHS (and hence RHS) is greater than 1.

506 Finally for all  $t > t_{\min}$ , where  $t_{\min} = \max(t_0, t_1)$ , we have,

$$\left( \frac{f(t)}{\Delta_i} \right)^{\frac{1}{g(t)}} \leq \left( e^{(\log \Phi(t))^{1-c}} \right)^{\log^c(\Phi(t))} = \Phi(t) \quad \forall t > t_{\min}$$

507  $\square$
