# Supplementary material for: Bandit algorithms: Letting go of logarithmic regret for statistical robustness
Source: arXiv:2006.12038 source file (2020-06-22)
Supplement: Supplementary file 3 [file appendix_upper_bounds_old.tex]

\section{Archive}


We first prove the concentration inequality for $\{\B, \SG, \G\}$ stated in Lemma \ref{bounded-conc-inequality}, \ref{subgaussian-conc-inequality} and \ref{heavytail-conc-inequality} respectively. These three lemma combined justifies property 1 of theorem \ref{general-upper-bound-thm} by setting $\delta=t^{-4}$

\subsection*{Proof of Lemma \ref{bounded-conc-inequality}}

Using Hoeffding's Inequality for bounded random variables, we get,
\begin{align*}
	\mathbb{P}\left(\frac{1}{u} \sum_{j=1}^{u}X_j - \mu \geq f(t) \sqrt{\frac{\log(\frac{1}{\delta})}{2u}}~\right) &\leq \text{exp}\left(-\frac{2u^2}{u(b-a)^2}f(t)^2 \frac{\log(\frac{1}{\delta})}{2u}\right)\\
	&= \text{exp}\left(- \log\left(\frac{1}{\delta}\right) \left( \frac{f(t)}{b-a}\right)^2\right)\\
	&\leq \delta \quad \text{for $t$ such that } f(t) > (b-a) \quad \QEDclosed
\end{align*}

\subsubsection*{Proof of Lemma \ref{subgaussian-conc-inequality}}

Using Concentration Inequality for $\sigma$-subgaussian random variables, we get,
\begin{align*}
	\mathbb{P}\left(\frac{1}{u} \sum_{i=1}^{u}X_i - \mu \geq f(t) \sqrt{\frac{2\log(\frac{1}{\delta})}{u}}\right) &\leq \text{exp}\left(-\frac{u}{2\sigma^2}f(t)^2 \frac{2\log(\frac{1}{\delta})}{u}\right)\\
	&= \text{exp}\left(- \log\left(\frac{1}{\delta}\right) \left( \frac{f(t)}{\sigma}\right)^2\right)\\
	&\leq \delta \quad \text{for $t$ such that } f(t) > \sigma \quad \QEDclosed
\end{align*}


\subsection*{Proof of concentration inequality for Sub exponential}

Statement
\begin{lemma}
Consider random variables $X_1, X_2, \dots, X_u \sim \SE$ which corresponds to samples drawn from $i^{th}$ arm. For sufficiently large $t$, if $~\U(i, u_i, t) > \U(j, u_j, t) ~ \forall j \neq i$, then with a probability less than $t^{-4}$, we have

$$\mu - \frac{1}{u} \sum_{i=1}^{u} X_i \geq \W(u, t) \quad \text{where} \W(u, t) = f(t) \sqrt{\frac{4\log(t)}{u}} $$

\end{lemma}

We first state a similar concentration inequality for $\SE(v, \alpha)$. We have,
$$\mathbb{P} \left( \frac{1}{u} \sum_{i=1}^{u} X_i - \mu \geq \W \right) \leq \exp \left(- \min \left \{ \frac{u \W^2}{2 v^2}, \frac{u\W}{2\alpha}  \right \} \right) $$

It is easy to see that the first term is the minimum for confidence widths less than $\W_0 = \frac{v^2}{\alpha}$. Now we claim that the above chosen confidence width will become less than $\W_0$ for sufficiently large $t$ for arms which are chosen at that large $t$. We argue this first in the sense of a different confidence window and then extend the argument to our confidence width of interest. Consider a confidence width $$ \W(u, n) = f(n) \sqrt{\frac{4\log(n)}{u}} .$$ where $n$ is a large number denoting the horizon. We see that here the confidence window is a strictly decreasing function with respect to the number of pulls of the arm $u$. Now, if arm $i$ is chosen for a large $t<n$, then the confidence window $\W(u_i, n)$ will be arbitrary close to $0$ and consequently less than $\W_0$. In addition, $\W(u, t)$ is strictly less than $\W(u, n)$. Thus, for sufficiently large $t$, if $~\U(i, u_i, t) > \U(j, u_j, t) ~ \forall j \neq i$, then $\W(u, t) < \W_0$. Hence we have,

\begin{align*}
    \mathbb{P} \left( \frac{1}{u} \sum_{i=1}^{u} X_i - \mu \geq f(t) \sqrt{\frac{4\log(t)}{u}} \right) &\leq \exp \left(- \frac{4 f(t)^2 \log(t)}{2v^2} \right)\\
    &\leq \exp(-4\log(t)) = t^{-4}
\end{align*}

where the last inequality holds because for large $t$, we have $f(t) > \sqrt{2}v$


\subsection*{Proof of Lemma \ref{heavytail-conc-inequality}}

This proof is similar to the ones presented in \citet{Yu2018PureEO} and \citet{bubeck}, but our concentration inequality is oblivious to the parameters $\epsilon$ and $B$. We state two propositions that will be required in the proof.
\begin{proposition} 
\label{prop-1}
For a random variable $X$ satisfying $\mathbb{E}[|X|^{1+\epsilon}] \leq B$, for any truncation $X_{max}$,
\begin{align*}
	\mathbb{E}[X \mathbbm{1}_{\left\{|X| > X_{max} \right\}}] \leq \frac{B}{X_{max}^{\epsilon}} \quad \text{and} \quad \mathbb{E}[X^2 \mathbbm{1}_{\left\{|X| \leq X_{max} \right\}}] \leq B X_{max}^{1-\epsilon}
\end{align*}
\end{proposition}
We have,
\begin{align*}
    \mathbb{E}[X_i \mathbbm{1}_{\left\{|X_i| > X_{max} \right\}}] \leq& ~~ \mathbb{E}[|X_i| \mathbbm{1}_{\left\{|X_i| > X_{max} \right\}}] \\
    =& ~~ \int_{B}^{\infty} |x| f(x) dx\\
    =& ~~ \int_{B}^{\infty} |x|^{1+\epsilon} |x|^{-\epsilon} f(x) dx \\
    =& ~~ X_{max}^{\epsilon} \int_{B}^{\infty} |x|^{1+\epsilon} f(x) dx \\
    \leq& ~~ X_{max}^{\epsilon} \mathbb{E}[|X|^{1+\epsilon}]\\
    \leq& ~~ \frac{B}{X_{max}^{\epsilon}}
\end{align*}
Similarly using $(1+\epsilon) + (1-\epsilon)=2$, we can prove the other inequality also.

\begin{proposition}
\label{prop-2}
	(\citet{selden2012}) Let $X_1, X_2, \dots , X_u$ be random variables satisfying $|X_i| \leq X_{max}, \mathbb{E}[X_i] = 0 \text{ and } \mathbb{E}[X_i] < \infty ~ \forall ~ i=1,2,\dots,u$. Then, with $1-\delta$ probability,
	\begin{align*}
	    \left|\sum_{i=1}^{u} X_i\right| \leq X_{max} \log\left(\frac{2}{\delta}\right) + \frac{1}{X_{max}} \sum_{i=1}^{u} \mathbb{E}[X_i^2]
	\end{align*}
\end{proposition}

Now to prove the lemma we have, for any truncation value $X_{max}$,
\begin{align*}
	\mu - \frac{1}{u} \sum_{i=1}^{u} X_i \mathbbm{1}_{\left\{|X_i|\leq X_{max} \right\}} &= \frac{1}{u} \sum_{i=1}^{u} \left( \mathbb{E}[X_i] - \mathbb{E}[X_i \mathbbm{1}_{\left\{|X_i|\leq X_{max} \right\}}] \right)\\ &+ \frac{1}{u} \sum_{i=1}^{u} \left( \mathbb{E}[X_i \mathbbm{1}_{\left\{|X_i|\leq _{max} \right\}}] - X_i \mathbbm{1}_{\left\{|X_i|\leq X_{max} \right\}} \right) \\
	&= \frac{1}{u} \sum_{i=1}^{u} \mathbb{E}[X_i \mathbbm{1}_{\left\{|X_i| > X_{max} \right\}}] \\ &+ \frac{1}{u} \sum_{i=1}^{n} \left( \mathbb{E}[X_i \mathbbm{1}_{\left\{|X_i|\leq X_{max} \right\}}] - X_i \mathbbm{1}_{\left\{|X_i|\leq X_{max} \right\}} \right)\\
	&\leq \frac{B}{X_{max}^{\epsilon}} + \frac{1}{u} \left\{ \ashutosh{2}X_{max} \log\left(\frac{2}{\delta}\right) + \frac{Bu}{\ashutosh{2}X_{max}^{\epsilon}}\right\} \qquad \text{with probability $1 - \delta$}\\
\end{align*}
\alternate{Below argument not correct since $X_{max} > 1$ is not guaranteed even for high $t$}

Here, the first term of the last statement follows from proposition \ref{prop-1} and the second term follows from proposition \ref{prop-2}. Now, choosing $X_{max} = \left( \frac{f(t)u}{\log\left(\frac{2}{\delta}\right)} \right)^{\frac{1}{1+g(t)}} $ and noting that $X_{max}>1, g(t)<\epsilon, $ and $f(t)>B$ for sufficiently large $t$, we get
\begin{align*}
    \mathbb{P}\left( \mu - \hat{\mu}_T \geq 4 f(t)^{\frac{1}{1+g(t)}} \left( \frac{\log(\frac{2}{\delta})}{u} \right)^{\frac{g(t)}{1+g(t)}} \right) \leq \delta
\end{align*}
where,
\begin{align*}
    \hat{\mu}_T = \frac{1}{u} \sum_{i=1}^{u} X_i \mathbbm{1}_{\left\{|X_i|\leq \left( \frac{f(t)u}{\log\left(\frac{2}{\delta}\right)} \right)^{\frac{1}{1+g(t)}} \right\}}
\end{align*}

\alternate{Now choose $X_{max}$ to be any increasing function f(t), which increases with number of rounds $t$. Then we have,}
\alternate{\begin{align*}
&\leq \frac{B}{f(t)^{\epsilon}} + \frac{1}{u} \left\{ f(t) \log\left(\frac{2}{\delta}\right) + \frac{Bu}{f(t)^{\epsilon}}\right\}
\end{align*}}
\alternate{\begin{align*}
&\leq \frac{2B}{f(t)^{\epsilon}} + f(t) \frac{\log\left(\frac{2}{\delta}\right)}{u}
\end{align*}}
\alternate{\begin{align*}
&\leq \frac{1}{\log(f(t))} + f(t) \frac{\log\left(\frac{2}{\delta}\right)}{u} \quad \forall ~ t>t_0
\end{align*}}
\alternate{Here, the last inequality holds since there exists a $t_0$ such that for all $t>t_0$, $2B\log(f(t)) < f(t)^{\epsilon}$}. This inequality will eventually hold since polynomial function will dominate logarithmic function in an asymptotic sense.



\subsubsection*{Proof of Theorem \ref{general-upper-bound-thm}}

After obtaining concentration bounds for the three classes of algorithms as given in property 1, we present a general proof for the expected number of times a sub-optimal arm is chosen given in property 2. The proof is similar to the bandit regret proof presented in \citet{bubeck}.

We define three events
\begin{align*}
	E_1&: \qquad \U(i^*, T_{i^*}(t-1), t) \leq \mu^*\\
	E_2&: \qquad \hat{\mu}(i, T_{i}(t-1), t) > \mu_i + \W(T_{i}(t-1), t)\\
	E_3&: \qquad \Delta_i < 2\W(T_{i}(t-1), t)
\end{align*}
for any sub-optimal arm $i$. Event $E_1$ occurs when optimal arm $i^*$ performs poorly, $E_2$ occurs when a sub-optimal arm $i$ performs well, and finally $E_3$ happens when a sub-optimal arm has not been pulled enough number of times.

\textbf{Claim:} If $i^{th}$ arm is chosen at time $t$, one of $E_1, E_2,$ or $ E_3$ is true.\\
\textbf{Proof:} We assume all of them to be false and show a contradiction. We have,
\begin{align*}
	\U(i^*, T_{i^*}(t-1), t) &> \mu^*\\
	&= \mu_i + \Delta_i\\
	&\geq \mu_i + 2\W(T_{i}(t-1), t)\\
	&\geq \hat{\mu}(i, T_{i}(t-1), t) + \W(T_{i}(t-1), t)\\
	&= \U(i, T_{i}(t-1), t)
\end{align*}
This is a contradiction since $i$ is chosen at time $t$.

Now, we use Lemmas \ref{bounded-conc-inequality}, \ref{subgaussian-conc-inequality} and \ref{heavytail-conc-inequality} as appropriate concentration inequality for $\B$, $\SG$ and $\G$ respectively. Now we have,
\begin{align*}
    \mathbb{P}(E_1) \leq& ~ \mathbb{P}(~\exists ~ s \in [t]: \U(i^*, s, t) \leq \mu^*) \qquad &\text{($s$ denotes the number of pulls of $i*$)}\\
    \leq& ~ t.t^{-4} = t^{-3} \qquad &\text{(union bound)}
\end{align*}
The above inequality holds for large $t$ ($t>t_{min}$). Similarly $\mathbb{P}(E_2) \leq t^{-3}$. Now,
\begin{align*}
	\mathbb{P}(E_1 \cup E_2) \leq \frac{2}{t^3}
\end{align*}
Let $u_i$ be a value of $T_i(t-1)$ for which $E_3$ is false. Then,
\begin{align*}
	\mathbb{E}[T_i(t)] &= \mathbb{E}\left[\sum_{s=1}^{t} \mathbbm{1}\{i^{th} \text{ arm is chosen at time } s\}\right]\\
	&\leq u_i + \mathbb{E}\left[\sum_{s=u_i+1}^{t} \mathbbm{1}\{i^{th} \text{ arm is chosen at time } s, E_{3} \text{ false}\}\right]\\
	&\leq u_i + \mathbb{E}\left[\sum_{s=u_i+1}^{t} \mathbbm{1}\{i^{th} \text{ arm is chosen at time } s, E_{1} \text{ or } E_{2} \text{ true}\}\right]\\
	&\leq u_i + \sum_{s=u_i+1}^{t} P(E_1 \cup E_2)\\
	&\leq u_i + \sum_{s=u_i+1}^{t} \frac{2}{s^3} \quad \leq u_i+4
\end{align*}
The last inequality is true only when $u_i>t_{min}$. As $t$ increases, $u_i$ will also increase but $t_{min}$ is constant with respect to the number of rounds. Hence, for large $t$, the above inequality will hold true. We choose the least possible $u_i$ to obtain tightest bound. Consequently,
$u_i$ is the minimum value value of $T_i(t-1)$ for which $\Delta_i > 2 \W(T_i(t-1), t)$ thus proving property 2. \ashutosh{Get rid of issues with constants}. Now, to finally prove the regret expression, we use the chosen value of confidence width $\W(T_i(t-1), t)$.

\textbf{Case 1: Regret upper bound for $\B$}

Solving for $u_i$ we get,
\begin{align*}
    \mathbb{E}[T_i(t)] \leq 8f(t)^2 \frac{\log(t)}{\Delta_i^2} + 4
\end{align*}
And hence,
\begin{align*}
    R_t(\pi_{\B}) &\leq \sum_{i:\Delta_i>0} \Delta_i \left(8f(t)^2 \frac{\log(t)}{\Delta_i^2} + 4 \right)\\
    &= \sum_{j:\Delta_j>0} \left( 4\Delta_i + 8f(t)^2 \frac{\log(t)}{\Delta_i} \right)
\end{align*}
which proves corollary \ref{bounded-regret-bound}.

\textbf{Case 2: Regret upper bound for $\SG$}

Solving for $u_i$ we get,
\begin{align*}
    \mathbb{E}[T_i(t)] \leq 32f(t)^2 \frac{\log(t)}{\Delta_i^2} + 4
\end{align*}
And hence,
\begin{align*}
    R_t(\pi_{\SG}) &\leq \sum_{i:\Delta_i>0} \Delta_i \left(32f(t)^2 \frac{\log(t)}{\Delta_i^2} + 4 \right)\\
    &= \sum_{j:\Delta_j>0} \left( 4\Delta_i + 32f(t)^2 \frac{\log(t)}{\Delta_i} \right)
\end{align*}
which proves corollary \ref{subgaussian-regret-bound}.

\textbf{Case 3: Regret upper bound for $\G$}

Solving for $u_i$ we get,
\begin{align*}
    \mathbb{E}[T_i(t)] \leq 8f(t)^{\frac{1}{g(t)}} \frac{\log(2t^4)}{\Delta_i^{\frac{1+g(t)}{g(t)}}} + 4
\end{align*}
And hence,
\begin{align*}
    R_t(\pi_{\G}) &\leq \sum_{i:\Delta_i>0} \Delta_i \left(8f(t)^{\frac{1}{g(t)}} \frac{\log(2t^4)}{\Delta_i^{\frac{1+g(t)}{g(t)}}} + 4 \right)\\
    &= \sum_{j:\Delta_j>0} \left( 4\Delta_i + 8\left(\frac{f(t)}{\Delta_i}\right)^{\frac{1}{g(t)}} \log(2t^4) \right)
\end{align*}
which proves corollary \ref{heavytail-regret-bound}.
